# Supplementary material for: Unusual Transport Properties with Non-Commutative System-Bath Coupling Operators
Source: arXiv:1907.11262 source file (2019-07-25)
Supplement: Supplementary file 1 [file SM_non_commutative_NESB_submit.pdf]

# Supplementary Materials for “Unusual Transport Properties with Non-Commutative System-Bath Coupling Operators”

Chenru Duan,<sup>1,2</sup> Chang-Yu Hsieh,<sup>2</sup> Junjie Liu,<sup>2</sup> and Jianshu Cao<sup>1,2,3,\*</sup>

*<sup>1</sup>Department of Chemistry, Massachusetts Institute of Technology,*

*77 Massachusetts Avenue, Cambridge, MA 02139*

*<sup>2</sup>Singapore-MIT Alliance for Research and Technology (SMART) Centre, Singapore 138602*

*<sup>3</sup>Beijing Computational Science Research Center, Beijing 100084, China*

## Abstract

In this Supplementary Materials, the detail derivation for the heat current expression by the extended hierarchy equation of motion and the non-equilibrium polaron-transformed Redfield equation are provided. The smooth transition for the heat current scaling dependence on the interaction strength from  $I \sim \alpha$  to  $I \sim \alpha^2$  is also presented.

---

\*Electronic address: [jianshu@mit.edu](mailto:jianshu@mit.edu)

## 1. EXTENDED HIERARCHY EQUATION OF MOTION

Consider a general total Hamiltonian consisting of a system, two baths and interaction parts,

$$H = H_S + \sum_{\nu=1,2} H_{B,\nu} + \sum_{\nu=1,2} V_\nu \otimes B_\nu, \quad (\text{S1})$$

where  $\nu$  labels two baths.  $H_{B,\nu} = \sum_j \omega_{\nu,j} b_{\nu,j}^\dagger b_{\nu,j}$  denotes the Hamiltonian for the bosonic bath, where  $b_{\nu,j}^\dagger$  ( $b_{\nu,j}$ ) is the creation (annihilation) operator.  $B_\nu = \sum_j g_{\nu,j} (b_{\nu,j}^\dagger + b_{\nu,j})$  is the bath operator.  $H_S$  denotes the system Hamiltonian and  $V_\nu$  is the coupling operator between system and  $\nu$ -th bath. Here we do not constrain the form of system-bath coupling operators so that  $V_1$  and  $V_2$  can be non-commutative. For simplicity, we consider a system-bath factorized initial condition,  $\rho_{\text{tot}}(0) = \rho_S(0) \otimes_\nu \rho_{B,\nu}^{\text{eq}}$ , where  $\rho_{B,\nu}^{\text{eq}} = \exp(-\beta_\nu H_{B,\nu}) / \text{Tr}\{\exp(-\beta_\nu H_{B,\nu})\}$  denotes the thermal equilibrium state of the bath.

Incorporating the counting field on the first bath, the Hamiltonian in Eq. (S1) becomes,

$$H[\frac{\chi}{2}] = H_S + \sum_{\nu=1,2} H_{B,\nu} + V_1 \otimes B_1[\frac{\chi}{2}] + V_2 \otimes B_2, \quad (\text{S2})$$

where  $O[\chi] = \exp(i\chi H_{B,1}) O \exp(-i\chi H_{B,1})$ . Then the cumulant generating function can be written as [1],

$$G(\chi, t) = \text{In} \left[ \text{Tr} \left\{ \exp(-iH[\frac{\chi}{2}]t) \rho_{\text{tot}}(0) \exp(iH[\frac{\chi}{2}]t) \right\} \right]. \quad (\text{S3})$$

The calculation of  $G(\chi, t)$  is equivalent with the propagation of reduced density matrix with  $H[\chi/2]$ ,

$$\rho_S(\chi, t) = \text{Tr}_B \left\{ \exp \left( -iH[\frac{\chi}{2}]t \right) \rho_{\text{tot}}(0) \exp \left( iH[\frac{\chi}{2}]t \right) \right\}, \quad (\text{S4})$$

so that  $G(\chi, t) = \text{In}[\text{Tr}_S\{\rho_S(\chi, t)\}]$  [2].

Hierarchy equation of motion (HEOM) calculate the dynamics of the reduced system with the facilitation of auxiliary fields [3, 4]. Here we use an extended HEOM in which more general bosonic baths can be treated with great accuracy [5, 6]. With the Wick's theorem, we have  $\tilde{\rho}_S(\chi, t) = \tilde{\mathcal{U}}_{\text{RMD}}(\chi, t)\rho_S(0, 0)$  in the interaction picture with

$$\tilde{\mathcal{U}}_{\text{RMD}}(\chi, t) = \mathcal{T}_+ \left\{ \exp \left( - \sum_{\nu, jk=0,1} \int_0^t ds \tilde{\mathcal{W}}_{\nu}^{jk}(\chi \delta_{1\nu}, s) \right) \right\}, \quad (\text{S5})$$

where  $\mathcal{T}_+$  is the time-ordering operator and  $\tilde{O}$  denotes an operator in the interaction picture.

The transition kernel is [2],

$$\tilde{\mathcal{W}}_{\nu}^{jk}(\chi \delta_{1\nu}, t) = \tilde{V}_{\nu}^j(t) \int_0^t ds \tilde{V}_{\nu}^k(s) C_{\nu}^{jk}(\chi \delta_{1\nu}, t-s). \quad (\text{S6})$$

Here only the transition kernel for the first bath ( $\tilde{\mathcal{W}}_1^{jk}(\chi, t)$ ) is dependent on  $\chi$  since we do not incorporate the counting field on the second bath. A superoperator notation  $O^0 A = OA$  and  $O^1 A = AO$  is used. The bath correlation with the counting field  $\chi$  can be calculated as,

$$\begin{aligned} C_{\nu}^{00}(\chi \delta_{1\nu}, t) &= C_{\nu}^{\text{R}}(t) + iC_{\nu}^{\text{I}}(t), \quad C_{\nu}^{10}(\chi, t) = -C_{\nu}^{\text{R}}(t - \chi \delta_{1\nu}) - iC_{\nu}^{\text{I}}(t - \chi \delta_{1\nu}), \\ C_{\nu}^{01}(\chi \delta_{1\nu}, t) &= -C_{\nu}^{\text{R}}(t + \chi \delta_{1\nu}) + iC_{\nu}^{\text{I}}(t + \chi \delta_{1\nu}), \quad C_{\nu}^{11}(\chi \delta_{1\nu}, t) = C_{\nu}^{\text{R}}(t) - iC_{\nu}^{\text{I}}(t). \end{aligned} \quad (\text{S7})$$

Here  $C_{\nu}^{\text{R}}(t)$  and  $C_{\nu}^{\text{I}}(t)$  are the real and imaginary part of the bath correlation function  $C_{\nu}(t) = 1/\pi \int_0^{\infty} d\omega J_{\nu}(\omega) [\coth \frac{\beta_{\nu}\omega}{2} \cos \omega t - i \sin \omega t]$  respectively.

According to the full counting statistics, the heat current is obtained,

$$\begin{aligned} I(t) &= \frac{\delta}{\delta t} \frac{\partial}{\partial i\chi} G(\chi, t)|_{\chi=0} \\ &= \text{Tr}_S \left\{ \frac{\delta}{\delta t} \frac{\partial}{\partial i\chi} \rho_S(\chi, t)|_{\chi=0} \right\} \end{aligned} \quad (\text{S8})$$

With  $\frac{\partial}{\partial \chi} C_\nu^X(t \pm \chi \delta_{1,\nu}) = \pm \delta_{1\nu} \frac{d}{dt} C_\nu^X(t) = \pm \delta_{1\nu} \dot{C}_\nu^X(t)$  and the transform of the coupling operators into the Liouville space, we have,

$$I(t) = -\text{Tr}_S\{\tilde{V}_1(t)\mathcal{T}_+[\int_0^t ds \dot{C}_1^R(t-s)(-i\tilde{\mathcal{L}}_{v,1}(s)) + \dot{C}_1^I(t-s)\tilde{\mathcal{S}}_{v,1}(s)\tilde{\mathcal{U}}_{\text{RMD}}(0,t)]\rho_S(0,0)\}, \quad (\text{S9})$$

where  $\tilde{\mathcal{L}}_{1,v}(t)O = [\tilde{V}_1(t), O]$  and  $\tilde{\mathcal{S}}_{1,v}(t)O = [\tilde{V}_1(t), O]_+$  are the commutator and anti-commutator in the Liouville space respectively. Note that none of the elements involved in Eq. (S9) are dependent on the counting field  $\chi$  as we take the limit  $\chi \rightarrow 0$  in Eq. (S8), so that the heat current can be calculated directly by the HEOM in which the original Hamiltonian Eq. (S1) is used.

In extended HEOM, bath correlation functions and their time derivative are simotinously decompsed with some function sets  $\{\phi_{\nu,j}^X(t)\}$ ,

$$C_\nu^X(t) = \sum_j a_{\nu,j}^X \phi_{\nu,j}^X(t),$$

$$\frac{\partial}{\partial t} C_\nu^X(t) = \sum_{j,j'} a_{\nu,j}^X \eta_{\nu,j,j'}^X \phi_{\nu,j'}^X(t), \quad (\text{S10})$$

where  $C_\nu^X(t)$  is the real ( $X = R$ ) or the imaginary ( $X = I$ ) part of the time correlation function of  $\nu$ -th bath. Here  $a_{\nu,j}^X$  are coefficients for the decomposition of  $C_\nu^X(t)$  and  $\eta_{\nu,j,j'}^X$  are the transition tensors for the time direvative of  $\phi_{\nu,j}^X(t)$ . With Eq. (S10), the auxiliary fields can be constructed and prapagated with an extended HEOM. [6]. Here we only present the construction of the first-order auxiliary fields which are directly involved in the heat current

expression, defined as

$$\begin{aligned}\sigma_1^{\vec{n}_\nu=(j)}(t) &= \mathcal{U}_S(t) \mathcal{T}_+ \left\{ \int_0^t ds \phi_{\nu,j}^R(t-s) (-i\tilde{\mathcal{L}}_{v,\nu}(s)) \tilde{\mathcal{U}}_{\text{RMD}}(t) \right\} \rho_S(0), \\ \sigma_1^{\vec{m}_\nu=(j)}(t) &= \mathcal{U}_S(t) \mathcal{T}_+ \left\{ \int_0^t ds \phi_{\nu,j}^I(t-s) \tilde{\mathcal{S}}_{v,\nu}(s) \tilde{\mathcal{U}}_{\text{RMD}}(t) \right\} \rho_S(0).\end{aligned}\quad (\text{S11})$$

Here  $\mathcal{U}_S(t) = \exp(-i\mathcal{L}_S t)$  transforms the operators back to the Schrodinger picture with the superoperator  $\mathcal{L}_S O = [H_S, O]$ . Plug Eq. (S10) and Eq. (S11) in to Eq. (S9), we can obtain the heat current expression of Eq. (3) in the main text.

## 2. SMOOTH TRANSITION FOR THE COUPLING STRENGTH DEPENDENCE ON THE HEAT CURRENT

The scaling relation between the heat current and the interaction strength is found altered with the change of system-bath coupling operators. At the extreme case where  $\theta = 0$ , we have  $I \sim \alpha^2$ , while  $I \sim \alpha$  at  $\theta = 0.5\pi$ , as shown in the main text. Here we demonstrate that there is a smooth transition for the scaling relation as we rotate  $\theta$  from 0 to  $0.5\pi$ . Consider the contribution of both terms in Eq. (4) in the main text, the heat current should be

$$I_{\text{fit}} = a \alpha + b \alpha^2, \quad (\text{S12})$$

where  $a = 0$  at  $\theta = 0$  and  $b = 0$  at  $\theta = 0.5\pi$ . In practical, the coefficients  $a$  and  $b$  can be obtained by the fitting from the numerical results of the extended HEOM at the weak coupling regime. In Table. S1, we present these coefficients for four different  $0 < \theta < 0.5\pi$ , where continuous change of both  $a$  and  $b$  can be observed. We find  $a$  ( $b$ ) increases as  $\theta$  increases (decreases) due to the increasing contribution of the  $\alpha$  ( $\alpha^2$ ). Figure S1 demonstrates

| $\theta(\pi)$ | $a(10^{-6})$ | $b(10^{-3})$ |
|---------------|--------------|--------------|
| 0.1           | 1.345        | 3.643        |
| 0.2           | 3.989        | 2.690        |
| 0.3           | 6.219        | 1.493        |
| 0.4           | 7.525        | 0.511        |

TABLE S1: The fitting coefficients  $a$  and  $b$  at different  $\theta$ . The fitting is done at the weak coupling limit ( $0.001 \leq \alpha \leq 0.005$ ). Other parameters are  $\Delta = 0.05$ ,  $T_1 = 1$  and  $T_2 = 0.9$ .

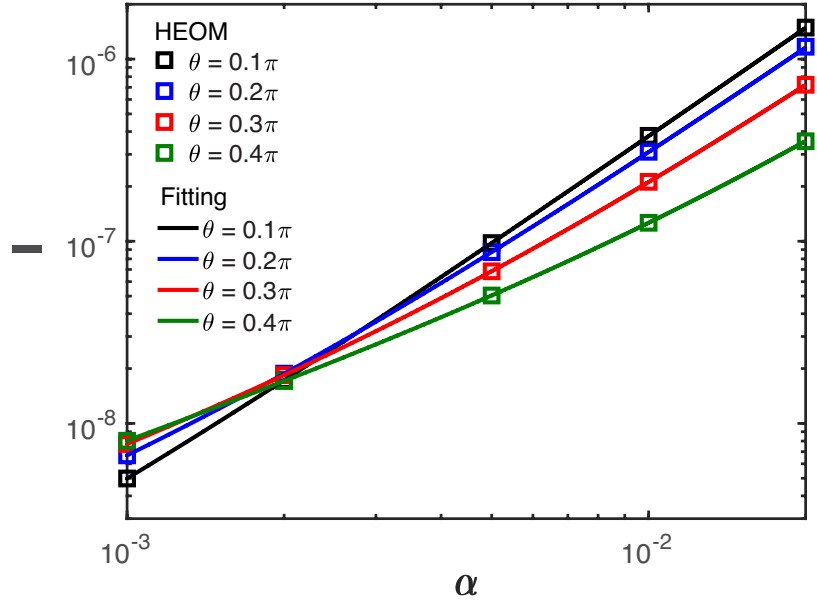

FIG. S1: Heat current  $I$  as a function of the coupling strength  $\alpha$  with different coupling operators to the second bath:  $\theta = 0.1\pi$  (black),  $\theta = 0.2\pi$  (blue),  $\theta = 0.3\pi$  (red) and  $\theta = 0.4\pi$  (green). Squares are results calculated the extended HEOM and solid lines are fitting results with Eq. (S12). Other parameters are the same as those in Table. S1.

the results of  $I_{\text{fit}}$  with the parameters in Table. S1, which agrees excellently with the heat current predicted by the extended HEOM.

### 3. NON-EQUILIBRIUM POLARON-TRANSFORMED REDFIELD EQUATION

We consider the Hamiltonian where  $\theta = 0$  in Eq. (1) in the main text,

$$H = \sigma_z \Delta + H_{B,1} + H_{B,2} + \sigma_x \sum_j g_{1,j} (b_{1,j}^\dagger + b_{1,j}) + \sigma_z \sum_j g_{2,j} (b_{2,j}^\dagger + b_{2,j}), \quad (\text{S13})$$

where  $H_{B,\nu} = \sum_j \omega_{\nu,j} b_{\nu,j}^\dagger b_{\nu,j}$  is the bath Hamiltonian. To calculate the heat current from a bath perspective, we incorporate the counting field  $\chi$  on the first bath, so Eq. (S14) becomes,

$$H = \sigma_z \Delta + H_{B,1} + H_{B,2} + \sigma_x \sum_j g_{1,j} (b_{1,j}^\dagger + b_{1,j}) + \sigma_z \sum_j g_{2,j} (b_{2,j}^\dagger [\frac{\chi}{2}] + b_{2,j} [\frac{\chi}{2}]), \quad (\text{S14})$$

where  $O[\chi] = \exp(i\chi H_{B,1}) O \exp(-i\chi H_{B,1})$ . For simplicity, we only displace the second bath with the polaron transformation  $U = \exp(-\sigma_z \sum_j g_{2,j} / \omega_{2,j} (b_{2,j}^\dagger - b_{2,j}))$ ,

$$\begin{aligned} H' &= U^\dagger H U \\ &= \Delta \sigma_z + \sum_\nu H_{B,\nu} + (\sigma_x \cosh 2A_2 \\ &\quad + i\sigma_y \sinh 2A_2) \sum_j g_{1,j} (b_{1,j}^\dagger [\frac{\chi}{2}] + b_{1,j} [\frac{\chi}{2}]) \end{aligned} \quad (\text{S15})$$

where  $A_2 = \sum_j g_{2,j} / \omega_{2,j} (b_{2,j}^\dagger - b_{2,j})$ . Then the Redfield equation can be written as

$$\frac{\partial}{\partial t} \rho_S(\chi, t) = -i[H_S, \rho_S(\chi, t)] - \int_0^\infty ds \text{Tr}_B \{ [H_{SB}[\chi], [H_{SB}[\chi](-s), \rho_S(\chi, t) \otimes \rho_B^{eq}]] \}. \quad (\text{S16})$$

Here  $H_{SB}[\chi] = (\sigma_x \cosh 2A_2 + i\sigma_y \sinh 2A_2) \sum_j g_{1,j} (b_{1,j}^\dagger [\frac{\chi}{2}] + b_{1,j} [\frac{\chi}{2}])$  is the system-bath interaction and  $H_S = \Delta \sigma_z$ . Writing Eq. (S16) into the Liouville space, we have  $\frac{\partial}{\partial t} \rho_S(\chi, t) = \mathcal{L} \rho_S(\chi, t)$  with

$$\mathcal{L} = \begin{bmatrix} L_{11} & L_{12} & 0 & 0 \\ L_{21} & L_{22} & 0 & 0 \\ 0 & 0 & L_{33} & L_{34} \\ 0 & 0 & L_{34} & L_{43} \end{bmatrix} \quad (\text{S17})$$

with each element  $L_{ij}$  written as

$$\begin{aligned}
L_{11} &= \eta^2 \int_0^\infty C_1(t) \exp(Q_2(t) + 2i\Delta t) + \eta^2 \int_0^\infty C_1(-t) \exp(Q_2(-t) - 2i\Delta t) \\
L_{22} &= \eta^2 \int_0^\infty C_1(t) \exp(Q_2(t) - 2i\Delta t) + \eta^2 \int_0^\infty C_1(-t) \exp(Q_2(-t) + 2i\Delta t) \\
L_{12} &= -\eta^2 \int_0^\infty C_1(t - \chi) \exp(Q_2(t) - 2i\Delta t) - \eta^2 \int_0^\infty C_1(-t - \chi) \exp(Q_2(-t) + 2i\Delta t) \\
L_{21} &= -\eta^2 \int_0^\infty C_1(t - \chi) \exp(Q_2(t) + 2i\Delta t) - \eta^2 \int_0^\infty C_1(-t - \chi) \exp(Q_2(-t) - 2i\Delta t) \\
L_{33} &= \eta^2 \int_0^\infty C_1(t) \exp(Q_2(t) + 2i\Delta t) + \eta^2 \int_0^\infty C_1(-t) \exp(Q_2(-t) + 2i\Delta t) - 2i\Delta \\
L_{44} &= \eta^2 \int_0^\infty C_1(t) \exp(Q_2(t) - 2i\Delta t) + \eta^2 \int_0^\infty C_1(-t) \exp(Q_2(-t) - 2i\Delta t) + 2i\Delta \\
L_{34} &= -\eta^2 \int_0^\infty C_1(t - \chi) \exp(-Q_2(t) - 2i\Delta t) - \eta^2 \int_0^\infty C_1(-t - \chi) \exp(-Q_2(-t) - 2i\Delta t) \\
L_{43} &= -\eta^2 \int_0^\infty C_1(t - \chi) \exp(-Q_2(t) + 2i\Delta t) - \eta^2 \int_0^\infty C_1(-t - \chi) \exp(-Q_2(-t) + 2i\Delta t)
\end{aligned} \tag{S18}$$

where  $C_1(t) = 1/\pi \int_0^\infty d\omega J_1(\omega) [\coth \frac{\beta_1 \omega}{2} \cos \omega t - i \sin \omega t]$  is the bath correlation function and  $Q_2(t) = 4/\pi \int_0^\infty J_2(\omega)/\omega^2 (n_2(\omega) \exp(i\omega t) + (n_2(\omega + 1) \exp(-i\omega t)))$  with  $n_2(\omega) = 1/(\exp(\beta_2 \omega) + 1)$  the Bose-Einstein distribution function. Here we have  $\eta = \exp(-4/\pi \int_0^\infty J_2(\omega)/\omega^2 (n(\omega) + 1/2)) \approx 1$  at the weak coupling regime.

The steady state heat current can be expressed with the minimal (ground state) eigenvalue as [7, 8],

$$\begin{aligned}
I &= \frac{\partial}{\partial i\chi} \min \{ \text{eig}(\mathcal{L}) \} \\
&= \frac{\frac{\partial}{\partial i\chi} L_{12}|_{\chi=0} L_{11} + \frac{\partial}{\partial i\chi} L_{21}|_{\chi=0} L_{22}}{L_{11} + L_{22}}.
\end{aligned} \tag{S19}$$

Substitute Eq. (S18) into Eq. (S19), we can obtain the heat current expression Eq. (6) in the main text. Note that higher order system-bath interaction are included by the polaron

transformation, so that the NE-PTRE successfully predict the heat current even when the system-bath coupling operators are non-commutative.

---

- [1] M. Esposito, U. Harbola, and S. Mukamel, *Rev. Mod. Phys.* **81**, 1665 (2009).
- [2] J. Cerrillo, M. Buser, and T. Brandes, *Phys. Rev. B* **94**, 214308 (2016).
- [3] Y. Tanimura, and R. Kubo, *J. Phys. Soc. Jpn.* **58**, 101 (1989).
- [4] Y. Tanimura, *J. Phys. Soc. Jpn.* **75**, 082001 (2006).
- [5] Z. Tang, X. Ouyang, Z. Gong, H. Wang, and J. Wu, *J. Chem. Phys.* **143**, 224112 (2015).
- [6] C. Duan, Z. Tang, J. Cao, and J. Wu, *Phys. Rev. B* **95**, 214308 (2017).
- [7] C. Wang, J. Ren, and J. Cao, *Sci. Rep.* **5**, 11787 (2015).
- [8] C. Wang, J. Ren, and J. Cao, *Phys. Rev. A* **95**, 023610 (2017).
